# Supplementary material for: SOCIA-$\nabla$: Textual Gradient Meets Multi-Agent Orchestration for Automated Simulator Generation
Source: arXiv:2505.12006 source file (2026-11-04)
Supplement: Supplementary file 1 [file 1_detailed_workflow.tex]

\begin{algorithm}[!htbp]
\caption{\socia Pipeline}
\label{alg:sociaworkflow}
\begin{algorithmic}[1]
\State \textbf{Inputs:} Full dataset $D$, task description $T$, role description $r$, task inputs $I$, ground-truth observables $Y$, Chain-of-Thought hints $\mathrm{CoT}$, hard constraints $\mathcal{C}$, Tolerance $\varepsilon_{\text{improve}}>0$
\State \textbf{Outputs:} $x^*$

\Statex
\State \textbf{Initialization}
\State $D_s \gets \textsc{BuildDataSchema}(D, T, I)$
\State $D \gets \textsc{DAA}(D_s, T, \mathrm{CoT})$  \Comment{DAA = Data Analysis Agent; Generate task brief based on the data schema and task description.}
\State $\text{best\_L} \gets +\infty,\quad \text{best\_x} \gets \text{None}$
\State $x_0 \gets f_{\mathrm{CGA}}(D, r)$ \Comment{CGA = Code Generation Agent; synthesize initial simulator $x$ from $D$ and $r$}
\State $t \gets 0,\quad \text{no\_improve} \gets 0$

\Statex
\State \textbf{Textual Gradient Optimization Loop}
\While{true}
  \State $o_t \gets f_{\mathrm{SEA}}(x_t, I)$ \Comment{SEA = Simulation Execution Agent; run simulator $x_t$ to obtain predictions $o_t$}
  \State $L_t \gets \ell(o_t, Y) + \lambda \sum_{j} \max\!\bigl(0,\, c_j(x_t)\bigr)$ \Comment{REA = Result Evaluation Agent; score fidelity and add constraint penalties}
  \State $g_t \gets \nabla_{\mathrm{LLM}}\!\left(x_t,\, o_t,\, \tfrac{\partial L_t}{\partial o_t}\right)$ \Comment{FGA = Feedback Generation Agent; textual gradients (critiques) to improve $x_t$}
  \State $m_t \gets \mathrm{Decay}_{\beta}(m_{t-1}) \;\oplus\; g_t$ \Comment{FGA merges historical critiques with current $g_t$}
  \State $\tilde{x}_{t+1} \gets \mathrm{TGD.step}(x_t,\, m_t;\ r)$ \Comment{CGA applies critiques to propose an unconstrained update}
  \State $x_{t+1} \gets \Pi_{\mathcal{C}}(\tilde{x}_{t+1})$ \Comment{CGA projects/repairs to satisfy hard constraints $\mathcal{C}$}

  \Statex \Comment{--- Early stopping with ``two-round no-improvement'' rule ---}
  \If{$L_t < \text{best\_L} - \varepsilon_{\text{improve}}$}
     \State $\text{best\_L} \gets L_t,\ \text{best\_x} \gets x_{t},\ \text{no\_improve} \gets 0$
  \Else
     \State $\text{no\_improve} \gets \text{no\_improve} + 1$
     \If{$\text{no\_improve} \ge 2$}
        \State \Return $\text{best\_x}$ \Comment{Exit if no lower loss for two consecutive rounds}
     \EndIf
  \EndIf

  \State $t \gets t + 1,\quad x_t \gets x_{t+1}$
\EndWhile

\end{algorithmic}
\end{algorithm}

This section details the end-to-end workflow of \socia and explains how the system instantiates TextGrad-style instance optimization over simulator code. We refer to Algorithm~\ref{alg:sociaworkflow} for the procedural view and unpack each stage below.

\paragraph{Inputs and Outputs}
\socia receives as inputs the full dataset $D$, a task description $T$, a role description $r$ (defining the expected interface/IO/semantics of the simulator), evaluation inputs $I$, ground-truth observables $Y$, CoT hints $\mathrm{CoT}$, the hard-constraint set $\mathcal{C}$ on code feasibility, and a user-defined tolerance $\varepsilon_{\text{improve}}>0$ for early stopping. The system returns a simulator program $x^*$ that minimizes the validation loss while satisfying $\mathcal{C}$.

\paragraph{Initialization}
\paragraph{Schema \& Brief Construction.}
\socia first constructs a data schema $D_s \gets \textsc{BuildDataSchema}(D, T, I)$ and then invokes the Data Analysis Agent (DAA) to produce a task brief tailored to the schema and task:
\[
D \gets \textsc{DAA}(D_s, T, \mathrm{CoT}),
\]
where $\mathrm{CoT}$ can encode structural hints, constraints and evaluation metrics.

\paragraph{One-shot Code Synthesis.}
Given the brief $D$ and role description $r$, the Code Generation Agent (CGA) synthesizes an initial simulator:
\[
x_0 \gets f_{\mathrm{CGA}}(D, r).
\]
We initialize the incumbent best objective and incumbent best code as $\text{best\_L} \gets +\infty$ and $\text{best\_x} \gets \text{None}$, and set the iteration counter $t \gets 0$ with a no-improvement counter $\text{no\_improve} \gets 0$.

\paragraph{Textual Gradient Optimization Loop}
At each iteration, \socia executes the following TextGrad-inspired loop that alternates (i) numeric execution and scoring, (ii) textual backpropagation of critiques, (iii) momentum-based aggregation of feedback, (iv) a textual gradient descent update, and (v) projection/repair to satisfy constraints.

\subsubsection{Numeric Execution (SEA)}
The Simulation Execution Agent (SEA) runs the current simulator on the evaluation inputs:
\[
o_t \gets f_{\mathrm{SEA}}(x_t, I),
\]
producing simulator outputs (e.g., trajectories, curves, logs, intermediate traces). SEA also surfaces execution metadata (runtime, determinism checks, exceptions) that later serves as evidence for textual feedback.

\subsubsection{Scoring with Constraint Penalties (REA)}
The Result Evaluation Agent (REA) computes a fidelity loss and augments it with constraint penalties:
\[
L_t \gets \ell(o_t, Y) + \lambda \sum_{j} \max\!\bigl(0,\, c_j(x_t)\bigr).
\]
Here $\ell(o_t,Y)$ quantifies closeness to the ground truth (e.g., MSE/MAE over curves, distributional distances, or task-specific metrics), while $c_j(x_t)$ measures violations of hard constraints (e.g., compilation, IO policy, determinism, output schema). The scalar $L_t$ is the objective optimized by the loop.

\subsubsection{Textual Gradient Generation (FGA)}
The Feedback Generation Agent (FGA) implements the textual backward operator by composing critiques conditioned on the forward context:
\[
g_t \gets \nabla_{\mathrm{LLM}}\!\Bigl(x_t,\, o_t,\, \tfrac{\partial L_t}{\partial o_t}\Bigr).
\]
Concretely, FGA assembles evidence from metric breakdowns, worst-case diffs between $o_t$ and $Y$, execution logs, determinism checks, and any failed constraint tests $\{c_j(x_t)>0\}$. The output $g_t$ is a set of localized, actionable code-edit suggestions that explain how to modify $x_t$ to reduce $L_t$ while satisfying $\mathcal{C}$.

\subsubsection{Textual Momentum}
To stabilize long-horizon editing and avoid cycling, \socia maintains a momentum buffer that exponentially decays historical critiques and merges them with the current gradient-like feedback:
\[
m_t \gets \mathrm{Decay}_{\beta}(m_{t-1}) \;\oplus\; g_t,
\]
where $\oplus$ denotes an ordered merge that preserves salient themes and avoids duplication. This textual momentum plays the role of a smoothed descent direction in code space.

\subsubsection{Textual Gradient Descent Update (CGA)}
CGA consumes the momentum-aggregated critiques and proposes an unconstrained update:
\[
\tilde{x}_{t+1} \gets \mathrm{TGD.step}(x_t,\, m_t;\ r).
\]
Operationally, \textsc{TGD.step} prompts the optimizer LLM with the current code $x_t$, the critique set $m_t$, and the role $r$, requesting a minimal, testable patch or a drop-in replacement that incorporates the critiques and preserves the intended interface/IO semantics.

\subsubsection{Projection / Repair to Feasibility}
To guarantee feasibility, the updated program is projected back to the constraint set:
\[
x_{t+1} \gets \Pi_{\mathcal{C}}(\tilde{x}_{t+1}),
\]
where $\Pi_{\mathcal{C}}$ is a textual projector realized by a constraint-repair routine that runs static checks, interface and determinism tests, and schema validators. Any failures are fed into a repair LLM that produces the smallest necessary edits until all $c_j(x_{t+1})\le 0$ (or the attempt budget is exhausted).

\paragraph{Early Stopping and Incumbent Tracking}
After scoring, \socia updates the incumbent best solution:
\[
\begin{aligned}
\text{if}\;& L_t < \text{best\_L} - \varepsilon_{\text{improve}} \\
\text{then}\;& \text{best\_L}\gets L_t,\ \text{best\_x}\gets x_t,\ \text{no\_improve}\gets 0.
\end{aligned}
\]
otherwise it increments the no-improvement counter. The loop terminates early if there is \emph{no strictly lower loss for two consecutive rounds}, at which point the system returns the current best program $\text{best\_x}$. Formally,
\[
\text{if}\ \text{no\_improve} \ge 2\ \text{ then return }\text{best\_x}.
\]

\paragraph{Putting It All Together}
For clarity, the iteration can be summarized as:
\[
\begin{aligned}
\textbf{Forward:}&\quad
o_t = f_{\mathrm{SEA}}(x_t, I),\\
&\quad L_t = \ell(o_t, Y) + \lambda \sum_{j} \max\!\bigl(0,\, c_j(x_t)\bigr).\\[2pt]
\textbf{Backward (text):}&\quad
g_t = \nabla_{\mathrm{LLM}}\!\Bigl(x_t,\, o_t,\, \tfrac{\partial L_t}{\partial o_t}\Bigr).\\[2pt]
\textbf{Momentum:}&\quad
m_t = \mathrm{Decay}_{\beta}(m_{t-1}) \oplus g_t.\\[2pt]
\textbf{Update:}&\quad
\tilde{x}_{t+1} = \mathrm{TGD.step}(x_t, m_t;\ r),\\
&\quad x_{t+1} = \Pi_{\mathcal{C}}(\tilde{x}_{t+1}).
\end{aligned}
\]

The loop proceeds with incumbent tracking and the two-round no-improvement stopping rule. This realizes TextGrad over a textual parameter~$x$ (the simulator program), combining numeric evidence with language-native critiques, momentum for stability, and projection for feasibility to deliver a robust and reproducible optimization of executable code.
