# Supplementary material for: SOCIA-$\nabla$: Textual Gradient Meets Multi-Agent Orchestration for Automated Simulator Generation
Source: arXiv:2505.12006 source file (2026-11-04)
Supplement: Supplementary file 2 [file 2_DAA_workflow.tex]

In this section, we present a detailed explanation of the underlying mechanism of \ofsocia \textbf{D}ata \textbf{A}nalysis \textbf{A}gent (\textbf{DAA}). We further elaborate on how the \textbf{DAA} conducts multidimensional relational mining to uncover latent interaction patterns among entities.

\begin{enumerate}[leftmargin=*]

    \item \textbf{Key Features}

    \textbf{Input Processing Paradigm}
    \begin{itemize}
        \item \textbf{Agent}: Takes \texttt{task\_description} and optional \texttt{task\_data}, building the task specification internally during processing.
    \end{itemize}

    \textbf{Workflow Integration}
    \begin{itemize}
        \item \textbf{Agent}: Combines task understanding and data analysis in a single step, returning a complete task specification with embedded analysis results.
    \end{itemize}

    \textbf{Template and Prompt Structure}
    \begin{itemize}
        \item \textbf{Agent}: Uses \texttt{templates/data\_analysis\_prompt.txt} with comprehensive simulation design framework.
    \end{itemize}

    \item \textbf{Workflow Analysis}

    \textbf{Core Process Method}
    
    The agent follows this workflow:
    \begin{lstlisting}[language=Python]
def process(
    self,
    task_description: str,
    task_data: Optional[Dict[str, Any]] = None,
    mode: str = "full",
    blueprint: Optional[Any] = None
) -> Dict[str, Any]:
\end{lstlisting}

    \textbf{Task Specification Building}
    
    The agent first constructs a comprehensive task specification:

    \textit{From Task Data (JSON)}
    \begin{itemize}
        \item Extracts \texttt{task\_objective} with description and simulation focus.
        \item Processes \texttt{data\_folder} and \texttt{data\_files} specifications.
        \item Incorporates \texttt{evaluation\_metrics} from the task file.
        \item Creates structured task specification with all necessary components.
    \end{itemize}

    \textit{From Task Description (String)}
    \begin{itemize}
        \item Creates minimal task specification when no JSON data is provided.
        \item Uses the description as the primary task objective.
        \item Sets default empty values for data files and evaluation metrics.
    \end{itemize}

    \textbf{Data Path Validation and File Discovery}
    \begin{itemize}
        \item Validates data path existence (raises \texttt{FileNotFoundError} if missing).
        \item Lists available files in the data directory.
        \item Supports multiple file types: CSV, JSON, GeoJSON, pickle, and Python files.
        \item Selects files for analysis based on task specification requirements.
    \end{itemize}
    
    \textbf{Schema Inference and Semantic Analysis}
    
    The agent implements sophisticated schema inference:

    \textit{CSV Schema Inference}
    \begin{itemize}
        \item Analyzes file structure using pandas.
        \item Captures data types, row/column counts, and sample data.
        \item Generates comprehensive data info using \texttt{df.info()}.
        \item Stores statistical summaries for numeric columns.
    \end{itemize}

    \textit{JSON Schema Inference}
    \begin{itemize}
        \item Handles both object and array structures.
        \item Analyzes data length and sample content.
        \item Captures value/item structure information.
        \item Provides type information for nested elements.
    \end{itemize}

    \textit{Semantic Summary Generation}
    \begin{itemize}
        \item Uses LLM to generate semantic metadata for each file.
        \item Contextualizes file content within the simulation task.
        \item Stores summaries directly in schema objects.
        \item Provides insights on how data should inform simulation entities.
    \end{itemize}

    \textbf{Comprehensive Analysis Prompt}
    
    The agent builds a sophisticated analysis prompt covering ten key areas:
    \begin{enumerate}
        \item \textbf{Overall Simulation Design}: Objective, initialization, execution, and outputs
        \item \textbf{Scale \& Granularity}: Time steps, spatial resolution, population size
        \item \textbf{Agent Archetypes}: Unit definitions, roles, attributes, and states
        \item \textbf{Interaction Topology}: Graph structures, layers, and protocols
        \item \textbf{Information Propagation}: Diffusion mechanisms and parameters
        \item \textbf{Exogenous Signals}: External interventions and effects
        \item \textbf{Action Decision Policy}: Role-specific decision functions
        \item \textbf{Holdout Plan}: Training/validation data splitting strategy
        \item \textbf{Simulation Evaluation}: Metrics and comparison methods
        \item \textbf{Calibratable Parameters}: Tunable parameters with bounds
    \end{enumerate}

    \textbf{LLM Analysis and Response Parsing}
    \begin{itemize}
        \item Calls LLM with comprehensive analysis prompt.
        \item Parses JSON response into structured format.
        \item Transforms response to match expected data analysis result structure.
        \item Handles parsing errors gracefully with fallback structures.
    \end{itemize}

    \item \textbf{Specialized Features}

    \textbf{Blueprint Integration}
    \begin{itemize}
        \item Designed to work with blueprint-based workflows.
        \item Supports blueprint mode processing.
        \item Integrates seamlessly with the code generation agent.
    \end{itemize}

    \textbf{File Type Support}
    \begin{itemize}
        \item \textbf{CSV Files}: Full statistical analysis with pandas integration.
        \item \textbf{JSON Files}: Structure analysis with type inference.
        \item \textbf{GeoJSON Files}: Special handling for geospatial data.
        \item \textbf{Pickle Files}: Network data and preprocessed objects.
        \item \textbf{Python Files}: Code analysis capabilities.
    \end{itemize}

    \textbf{Semantic Metadata Generation}
    \begin{itemize}
        \item LLM-powered semantic analysis of file content.
        \item Context-aware summaries based on task description.
        \item Integration guidance for simulation entities.
        \item Relationship identification between data elements.
    \end{itemize}

    \textbf{Comprehensive Output Structure}
    
    The agent returns a complete task specification with:
    \begin{itemize}
        \item \texttt{data\_analysis\_result}: Structured analysis covering all ten areas
        \item \texttt{file\_summaries}: Formatted file information with semantic summaries
        \item \texttt{schemas}: Detailed file schemas with metadata
        \item Original task specification components
    \end{itemize}
    
    \item \textbf{Configuration and Usage}

    \textbf{Configuration}
    \begin{lstlisting}[language=yaml]
data_analysis:
  enabled: true
  prompt_template: "templates/data_analysis_prompt.txt"
  output_format: "json"
  supported_data_types: ["csv", "json", "geojson", "shapefile"]
\end{lstlisting}

    \textbf{Dependency Injection}
    \begin{itemize}
        \item Registered in \texttt{AgentContainer} as \texttt{data\_analysis\_agent}.
        \item Available through workflow manager agent providers.
        \item Configured with output path for result persistence.
    \end{itemize}

    \textbf{Integration Points}
    \begin{itemize}
        \item Works with the task understanding agent.
        \item Integrates with the code generation agent.
        \item Supports blueprint-based workflows.
        \item Used in test workflows for data analysis and code generation.
    \end{itemize}

    \item \textbf{Technical Implementation Details}

    \textbf{Error Handling}
    \begin{itemize}
        \item Comprehensive file validation with clear error messages.
        \item Graceful handling of missing files and parsing errors.
        \item Fallback structures for LLM response parsing failures.
        \item Detailed logging for debugging and monitoring.
    \end{itemize}

    \textbf{Data Processing}
    \begin{itemize}
        \item Efficient file scanning with type detection.
        \item Memory-conscious data loading for large files.
        \item Statistical analysis with pandas integration.
        \item Schema inference without loading entire datasets.
    \end{itemize}

    \textbf{LLM Integration}
    \begin{itemize}
        \item Structured prompt building with template integration.
        \item JSON response parsing with error recovery.
        \item Semantic analysis for contextual understanding.
        \item Fallback handling for malformed responses.
    \end{itemize}

    \item \textbf{Use Cases and Applications}

    \textbf{Blueprint-Based Simulation Development}
    \begin{itemize}
        \item Ideal for structured simulation design workflows.
        \item Supports complex multi-agent system analysis.
        \item Handles calibration and validation data preparation.
    \end{itemize}

    \textbf{Comprehensive Data Analysis}
    \begin{itemize}
        \item Provides end-to-end analysis from task description to simulation design.
        \item Combines data understanding with simulation parameter extraction.
        \item Supports multiple file formats and data structures.
    \end{itemize}

    \textbf{Iterative Development}
    \begin{itemize}
        \item Integrates with feedback-driven workflows.
        \item Maintains consistency across development iterations.
        \item Supports blueprint updates and modifications.
    \end{itemize}

    \item \textbf{Summary}

    The \textbf{Data Analysis Agent} represents a sophisticated, blueprint-focused approach to data analysis within the SOCIA system. Its key distinguishing features include:
    \begin{enumerate}
        \item \textbf{Integrated task specification building} that combines task understanding and data analysis
        \item \textbf{Advanced schema inference} with semantic analysis using LLM capabilities
        \item \textbf{Comprehensive simulation design framework} covering all aspects of model construction
        \item \textbf{Blueprint-based workflow integration} optimized for structured simulation development
        \item \textbf{Multi-format data support} with specialized handling for various file types
        \item \textbf{End-to-end analysis} from raw data to simulation parameter extraction
    \end{enumerate}

    This agent serves as an alternative to the regular data analysis agent, providing enhanced capabilities for complex simulation scenarios that require comprehensive data understanding, structured analysis, and seamless integration with blueprint-based development workflows. It is particularly well-suited for scenarios where data analysis needs to be tightly coupled with simulation design and parameter calibration processes.

\end{enumerate}
