# Supplementary material for: SOCIA-$\nabla$: Textual Gradient Meets Multi-Agent Orchestration for Automated Simulator Generation
Source: arXiv:2505.12006 source file (2026-11-04)
Supplement: Supplementary file 3 [file 3_cga.tex]

In this section, we describe the \textbf{C}ode \textbf{G}eneration \textbf{A}gent (\textbf{CGA}) workflow in the \socia framework.

The \textbf{CGA} is responsible for transforming conceptual model plans into executable \texttt{Python} code for simulations. 
Its operation can be broken down into two major phases, i.e., \textit{Initial Code Generation} phase and \textit{Self-Checking and Improvement Loop} phase.

\subsection{Phase 1: Initial Code Generation}
\label{ssec:initial_code_CGA}
When the agent is invoked through its \texttt{process} method, it follows these steps:

\begin{enumerate}
    \item \textbf{Input Processing}: The agent receives key inputs including:
    \begin{itemize}
        \item \verb|task_spec|: Detailed requirements for the simulation.
        \item \verb|model_plan|: The conceptual model design from the \textbf{Model Planning Agent}.
        \item \verb|data_analysis|: Results from data analysis.
        \item \verb|feedback|: Feedback from previous iterations.
        \item \verb|historical_fix_log|: Log of issues and fixes from previous iterations.
    \end{itemize}

    \item \textbf{Prompt Construction}: The agent builds a comprehensive prompt using \verb|_build_prompt()|:
    \begin{lstlisting}[language=Python]
       prompt = self._build_prompt(
           task_spec=task_spec,
           model_plan=model_plan,
           data_analysis=data_analysis,
           feedback=feedback,
           data_path=data_path,
           previous_code=previous_code
       )
    \end{lstlisting}
    This prompt is constructed from a template file (as shown in Prompt~\ref{prompt:code_generation}), which provides detailed instructions to the LLM about how to generate the code, including specific requirements for simulation code structure, class implementations, and coding standards.

    \item \textbf{Code Generation}: The agent calls the LLM to generate code: 
    \begin{lstlisting}[language=Python]
      llm_response = self._call_llm(prompt)
    \end{lstlisting}

    \item \textbf{Code Extraction}: The generated code is extracted from the LLM response: 
    \begin{lstlisting}[language=Python]
    code = self._extract_code(llm_response)
    code = self._strip_markdown_fences(code)
    \end{lstlisting}
    The agent looks for code blocks marked with \verb|```python| and \verb|```| delimiters, and extracts the content. If no delimiters are found, it assumes the entire response is code.

    \item \textbf{Feedback Application}: If specific code snippets are included in feedback, the agent applies them directly:
    \begin{lstlisting}[language=Python]
       if feedback and 'code_snippets' in feedback:
       for snippet in feedback['code_snippets']:
           before = snippet.get('before', '')
           after = snippet.get('after', '')
           if before and after and before in code:
               code = code.replace(before, after)
    \end{lstlisting}

    \item \textbf{Basic Code Fixes}: The agent performs basic error corrections:
    \begin{lstlisting}[language=Python]
          code = self._fix_unclosed_docstrings(code)
    \end{lstlisting}
    This handles common issues like unbalanced triple-quoted docstrings.
\end{enumerate}

\subsection{Phase 2: Self-Checking and Improvement Loop}
\label{ssec:self_checking_loop_CGA}

After generating the initial code, the agent enters a sophisticated self-improvement cycle using the \verb|_run_self_checking_loop| method. This is where the agent becomes truly agentic by evaluating and improving its own output:
\begin{lstlisting}[language=Python]
    code = self._run_self_checking_loop(
    code=code,
    task_spec=task_spec,
    model_plan=model_plan,
    feedback=feedback,
    historical_fix_log=historical_fix_log
)
\end{lstlisting}

The self-checking loop operates for up to three iterations (controlled by \verb|max_attempts|), performing these steps in each iteration:

\begin{enumerate}
    \item \textbf{Comprehensive Code Quality Check}: The agent analyzes the code for quality issues using \verb|_perform_code_quality_check()|:
    \begin{lstlisting}[language=Python]
    issues.extend(self._perform_code_quality_check(improved_code, task_spec, model_plan))
    \end{lstlisting}
    This check looks for:
    \begin{itemize}
        \item Syntax errors and potential runtime errors
        \item Placeholder functions (those with just 'pass')
        \item Unimplemented methods or functionality
        \item Inconsistencies between the model plan and implementation
        \item Inefficient code or algorithms
        \item Poor error handling
        \item Lack of type annotations
        \item Missing documentation
    \end{itemize}

    \item \textbf{Feedback Implementation Check}: If feedback exists from previous iterations, the agent verifies that all required fixes have been implemented:
    \begin{lstlisting}[language=Python]
       if feedback:
           issues.extend(self._check_feedback_implementation(improved_code, feedback))
    \end{lstlisting}

    \item \textbf{Historical Issues Check}: The agent checks if the code reintroduces issues that were fixed in previous iterations:
    \begin{lstlisting}[language=Python]
    if historical_fix_log:
        issues.extend(self._check_historical_issues(improved_code, historical_fix_log))
    \end{lstlisting}

    \item \textbf{Issue Resolution}: If any issues are found, the agent improves the code:
    \begin{lstlisting}[language=Python]
    if issues:
       # Collect relevant fixed_log entries for reference
       fixed_log_references = self._collect_fixed_log_references(issues, historical_fix_log)
       
       # Improve the code based on issues and fixed_log references
       improved_code = self._improve_code_based_on_issues(
           code=improved_code,
           issues=issues,
           fixed_log_references=fixed_log_references,
           task_spec=task_spec,
           model_plan=model_plan
       )
    \end{lstlisting}
    This improvement process sends another prompt to the LLM with detailed information about the issues and how to fix them, and applies the resulting improved code.

    \item \textbf{Final Syntax Verification}: After each improvement iteration, the agent verifies the code has valid syntax:
    \begin{lstlisting}[language=Python]
    try:
       compile(improved_code, '<improved>', 'exec')
       self.logger.info("Improved code passed syntax check")
   except SyntaxError as err:
       self.logger.warning(f"Syntax error in improved code: {err}")
       # If this is the last attempt, we should at least make sure the code compiles
       if attempt == max_attempts - 1:
           improved_code = self._fix_syntax(improved_code, err)
    \end{lstlisting}

    \item \textbf{Loop Termination}: The loop terminates when either:
    \begin{itemize}
        \item No issues are found in an iteration
        \item The maximum number of attempts (3) is reached
    \end{itemize}
    
\end{enumerate}

\subsection{Final Output Preparation}
\label{ssec:final_output_preparation}
After the self-checking loop completes, the agent:
\begin{enumerate}
    \item \textbf{Generates a Code Summary}: Creates a summary of the final code: 
    \begin{lstlisting}[language=Python]
    code_summary = self._generate_code_summary(code)
    \end{lstlisting}

    \item \textbf{Performs Final Syntax Check}: Ensures the code is syntactically correct:
    \begin{lstlisting}[language=Python]
    try:
       compile(result['code'], '<generated>', 'exec')
   except SyntaxError as err:
       # Attempt final auto-fix via LLM if there's still a syntax error
       # ...
    \end{lstlisting}

    \item \textbf{Returns the Result}: The agent returns a structured result containing:
    \begin{lstlisting}[language=Python]
    result = {
       "code": code,
       "code_summary": code_summary,
       "metadata": {
           "model_type": model_plan.get("model_type", "unknown"),
           "entities": [e.get("name") for e in model_plan.get("entities", [])],
           "behaviors": [b.get("name") for b in model_plan.get("behaviors", [])]
       }
   }
    \end{lstlisting}
\end{enumerate}

The \textbf{CGA} exemplifies sophisticated AI-driven code generation with built-in quality assurance. By incorporating a self-improvement loop, the agent mimics human programmer behavior of writing code, reviewing it, and making improvements before finalizing it. This process produces higher quality code that aligns with the conceptual model and incorporates feedback from previous iterations when available.
