# Supplementary material for: SOCIA-$\nabla$: Textual Gradient Meets Multi-Agent Orchestration for Automated Simulator Generation
Source: arXiv:2505.12006 source file (2026-11-04)
Supplement: Supplementary file 4 [file 4_fga.tex]

In this section, we describe the \textbf{F}eedback \textbf{G}eneration \textbf{A}gent (\textbf{FGA}) workflow in the \socia framework.

The \textbf{FGA} serves as the critical evaluative component in the \socia framework's iterative improvement cycle. 
It synthesizes information from multiple sources to provide structured, actionable feedback for improving simulation code. 
Here's how it works:

\paragraph{1. Setup and Initialization.} 
The agent begins with initialization that establishes its fundamental environment:
\begin{lstlisting}[language=Python]
def __init__(self, config: Dict[str, Any] = None, output_path: Optional[str] = None):
    # Set default config if none provided
    if config is None:
        config = {
            "prompt_template": "templates/feedback_generation_prompt.txt",
            "output_format": "json"
        }
    
    super().__init__(config)
    
    # Set output path
    self.output_path = output_path or os.getcwd()
    
    # Set template directory path
    self.template_dir = os.path.join(
        os.path.dirname(os.path.dirname(os.path.dirname(os.path.abspath(__file__)))),
        "templates"
    )
\end{lstlisting}
This setup is critical as it points to the feedback generation prompt template and establishes the directory structure for related operations.

\paragraph{2. Core Feedback Generation Process.} 
When invoked, the agent's \verb|process| method coordinates the entire feedback generation workflow:

\begin{lstlisting}[language=Python]
def process(self, task_spec, verification_results, simulation_results, 
           evaluation_results, model_plan, generated_code, 
           current_code, previous_code, iteration, 
           historical_fix_log):
\end{lstlisting}
The process follows these key steps:
\begin{itemize}
    \item \textbf{Step 1: Generate Code Diff for Context}. If both previous and current code versions are available, the agent creates a diff to understand what has changed between iterations:
    \begin{lstlisting}[language=Python]
    if previous_code and current_code:
        prev_lines = previous_code.splitlines(keepends=True)
        curr_lines = current_code.splitlines(keepends=True)
        
        diff = difflib.unified_diff(
            prev_lines, curr_lines,
            fromfile=f"simulation_code_iter_{iteration-1}.py",
            tofile=f"simulation_code_iter_{iteration}.py",
            n=3  # Context lines
        )
        code_diff = "".join(diff)
    \end{lstlisting}
    This diff provides critical context for understanding how the code has evolved and whether previous feedback was incorporated.

    \item \textbf{Step 2: Update Historical Fix Log.} 
    Before generating new feedback, the agent checks if previously identified issues have been fixed in the current code:
    \begin{lstlisting}[language=Python]
    if iteration > 0 and historical_fix_log and current_code:
        self._check_fixed_issues(historical_fix_log, current_code, iteration)
    \end{lstlisting}
    This check uses a specialized prompt (\verb|_build_fix_check_prompt|, as shown in Prompt~\ref{ssec:fix_check_prompt}) that compares the current code against previously documented issues to determine if they've been resolved.

    \item \textbf{Step 3: Generate Comprehensive Feedback.} 
    The agent uses the BaseAgent's \verb|_build_prompt| method which fills a template with all the available information. The template (\verb|feedback_generation_prompt.txt|, as shown in Prompt~\ref{prompt:feedback_generation}) is structured to guide the LLM to perform a comprehensive analysis with the following workflow:

    \begin{enumerate}
        \item \textbf{Code Analysis}: The LLM examines the current code and recent changes for:
        \begin{itemize}
            \item Logical errors in the implementation
            \item Specific syntactic or semantic errors
            \item Execution flow issues
            \item Appropriateness of data structures and algorithms
            \item Issues with dependencies
        \end{itemize}

        \item \textbf{Results Integration}: The feedback incorporates:
        \begin{itemize}
            \item Verification results from code static analysis
            \item Simulation execution results
            \item Evaluation results comparing simulation output to expected behavior
        \end{itemize}

        \item \textbf{Structured Output Generation}: The feedback is structured as a JSON object with:
        \begin{itemize}
            \item \verb|summary|: Brief overview of the feedback.
            \item \verb|critical_issues|: Issues that must be addressed.
            \item \verb|model_improvements|: Conceptual improvements to the simulation model.
            \item \verb|code_improvements|: Specific code modifications
            \item \verb|data_alignment_suggestions|: Ways to align the simulation with real-world data
            \item \verb|prioritized_actions|: Ordered list of recommended next steps.
            \item \verb|code_snippets|: Specific before/after code examples.
        \end{itemize}
    \end{enumerate}

    \item \textbf{Step 4: Response Parsing and Validation.} After receiving the LLM's response, the agent processes it:
    \begin{lstlisting}[language=Python]
    # Parse the LLM response and validate required schema fields
    parsed = self._parse_llm_response(llm_response)
    if not isinstance(parsed, dict) or "summary" not in parsed:
        self.logger.warning("LLM feedback format is invalid, using placeholder feedback")
        feedback = self._create_placeholder_feedback()
    else:
        feedback = parsed
    \end{lstlisting}
    If the LLM's response doesn't meet the expected format, a placeholder feedback structure is provided to ensure the workflow doesn't break.
\end{itemize}

\paragraph{3. Historical Issue Tracking.} 
A unique feature of the Feedback Generation Agent is its historical issue tracking mechanism:
\begin{lstlisting}[language=Python]
    def _check_fixed_issues(self, historical_fix_log, current_code, current_iteration):
    # Create prompt to check fixed issues
    prompt = self._build_fix_check_prompt(historical_fix_log, current_code, current_iteration)
    
    # Call LLM to analyze fixes
    llm_response = self._call_llm(prompt)
    
    # Parse response and update historical fix log
    fixed_issues = self._parse_fix_check_response(llm_response)
    if fixed_issues:
        for iteration_key, issues in fixed_issues.items():
            for fixed_issue in issues:
                if fixed_issue.get("status") == "fixed":
                    # Update status in historical log
                    # ...
\end{lstlisting}

This system:
\begin{itemize}
    \item Maintains a record of issues across iterations.
    \item Uses the LLM to determine if each issue has been fixed in the current code.
    \item Updates the historical log with the status of each issue.
    \item Provides this context to future iterations to prevent re-introducing fixed issues.
\end{itemize}
The agent takes special care to handle the JSON parsing of LLM responses, with multiple fallback strategies to ensure robust operation even when responses are imperfectly formatted.

\paragraph{4. Output Generation.}
The final output is a comprehensive feedback structure that guides the Code Generation Agent in creating improved code for the next iteration. The feedback includes:
\begin{itemize}
    \item Critical issues that need immediate attention.
    \item Model improvements for better simulation accuracy.
    \item Code improvements with specific snippets demonstrating the changes.
    \item Data alignment suggestions to better match real-world behavior.
    \item A prioritized action plan.
\end{itemize}

This structured feedback creates a clear roadmap for the next iteration, enabling continuous improvement of the simulation over time.

The \textbf{FGA}'s sophisticated approach to analyzing code, tracking issues over time, and providing structured, actionable feedback is central to \ofsocia ability to iteratively improve simulations through a multi-agent workflow.
