# Supplementary material for: SOCIA-$\nabla$: Textual Gradient Meets Multi-Agent Orchestration for Automated Simulator Generation
Source: arXiv:2505.12006 source file (2026-11-04)
Supplement: Supplementary file 5 [file 5_code_evol.tex]

\subsection{Analysis of the functionalities of different stages of the applications}
\label{ssec:functionalities_different_stage}
In this section, we analyze the code generated for the three applications discussed in the main text—\textbf{e-Commerce and Retail User Modeling (User)}, \textbf{Personal Mobility Generation (Mobility)}, and \textbf{Mask Adoption Behavior (Mask)}—to illustrate how \socia autonomously evolves simulation code for Cyber-Physical-Social (CPS) systems through its feedback-loop mechanism. This iterative process not only reveals the \textbf{pace of code evolution}—i.e., what core functionalities typically emerge by a given iteration—but more importantly, it demonstrates \socia's ability to \textbf{self-evaluate and optimize code} over successive iterations.

\begin{table*}[h]
    % \caption{Summary of differences between \libName and other related multi-agent systems.  \textbf{infrastructure}: whether the system is designed as a generic infrastructure for building LLM applications. \textbf{conversation pattern}: the types of patterns supported by the implemented systems. Under the `static’ pattern, agent topology remains unchanged regardless of different inputs. \libName allows flexible conversation patterns, including both static and dynamic patterns that can be customized based on different application needs.  
    % \textbf{execution-capable}: whether the system can execute LLM-generated code; \textbf{human involvement}: whether (and how) the system allows human participation during the execution process of the system. \libName allows flexible human involvement in multi-agent conversation with the option for humans to skip providing inputs. 
    % }
    \caption{
    Summary of the functionalities achieved by the generated code at different stages (\textbf{iterations}) across various applications. \textbf{Blank cells} in the table indicate functionalities that \textbf{were not successfully implemented}.
    In terms of naming of \textbf{Code}, the format follows \textbf{Application-Number}, such as ``User-0'', which represents the simulator generated for the \textit{User Modeling Task} at \textit{}{Iteration 0}.
    }
    \label{tab:simulation_code_iteration}
    \small
        \begin{tabular}{p{1.4cm}|P{1.66cm}P{1.66cm}P{1.66cm}P{1.66cm}P{1.66cm}P{1.66cm}}
            \hline %\hline
           Code & Writing component classes & Building the simulator framework & Error Handling & Visuali-zation  & Parameter calibration & Model refinement  \\ \hline
            User-0 & \cmark &   &  &     &  &   \\
            User-1 & \cmark & \cmark  &  &     &  &   \\
            User-2 & \cmark & \cmark  & \cmark &     &  &   \\
            User-3 & \cmark & \cmark  & \cmark & \cmark    &  &   \\
            User-4 & \cmark & \cmark  & \cmark &  \cmark   & \cmark &   \\
            User-5 & \cmark & \cmark  & \cmark &  \cmark   & \cmark & \cmark  \\
            \hline
            Mobility-0 & \cmark & \cmark  &  &     &  &   \\
            Mobility-1 & \cmark & \cmark  & \cmark &  \cmark   &  &   \\
            Mobility-2 & \cmark & \cmark  & \cmark &  \cmark   & \cmark &   \\
            Mobility-3 & \cmark & \cmark  & \cmark &  \cmark   & \cmark & \cmark  \\
            \hline
            Mask-0 & \cmark & \cmark  &  &     &  &   \\
            Mask-1 & \cmark & \cmark  & \cmark &     &  &   \\
            Mask-2 & \cmark & \cmark  & \cmark &  \cmark   &  &   \\
            Mask-3 & \cmark & \cmark  & \cmark &  \cmark   &  &   \\
            Mask-4 & \cmark & \cmark  & \cmark &  \cmark   & \cmark &   \\
            Mask-5 & \cmark & \cmark  & \cmark &  \cmark   & \cmark & \cmark  \\
            \hline
        \end{tabular}
\end{table*}

As shown in the Table~\ref{tab:simulation_code_iteration}, we summarize the functionalities that have been implemented or remain unimplemented at various iterations across different applications. This comparison offers an intuitive view of how the generated code progressively evolves toward satisfying the simulation objectives.

Also, based on the analysis of Table~\ref{tab:simulation_code_iteration}, several notable findings emerge regarding the iterative evolution of simulation code generated by \socia across the three applications:

\begin{enumerate}
    \item \textbf{Progressive Feature Accumulation Across Iterations.} Each application exhibits a clear trend of \textbf{increasing functionality} over successive iterations. Initial iterations primarily focus on foundational capabilities—such as writing component classes and constructing the simulator framework—while later iterations incorporate more advanced features such as visualization, parameter calibration, and model refinement.
    \begin{itemize}
        \item For example, in the \textbf{User Modeling} application, visualization appears only at \textit{Iteration 3 and beyond}, while parameter calibration and model refinement are introduced at \textit{Iterations 4 and 5}, respectively.
        \item A similar pattern is observed in the \textbf{Personal Mobility Generation} and \textbf{Mask Adoption Behavior}, suggesting that \socia consistently applies a staged development process that begins with infrastructure and proceeds toward higher-level analytical functions.
    \end{itemize}

    \item \textbf{Delayed Emergence of Advanced Capabilities.} Advanced features such as \textbf{parameter calibration} and \textbf{model refinement} are consistently absent from early iterations (e.g., \textit{User-0}, \textit{Mobility-0}, \textit{Mask-0}) and only emerge in later stages.
    \begin{itemize}
        \item This implies that these functions require prior structural and semantic foundations to be in place, and their emergence is likely contingent on successful completion of earlier components and feedback integration.
    \end{itemize}

    \item \textbf{Error Handling Appears as an Intermediate Milestone.} Across all applications, \textbf{error handling} tends to appear in the \textit{second or third iteration}, suggesting that initial versions of the code often contain syntactic or structural issues, which are only systematically addressed after a basic simulation flow has been established.
    \begin{itemize}
        \item For instance, error handling is implemented starting from \textit{User-2}, \textit{Mobility-1}, and \textit{Mask-1}.
    \end{itemize}

    \item \textbf{Variation in Evolution Pace Across Applications.} While the general trend of progressive refinement holds across all three applications, the \textbf{pace of evolution differs}:
    \begin{itemize}
        \item The \textbf{User Modeling} application demonstrates a faster progression, achieving full functionality by \textit{Iteration 5}.
        \item The \textbf{Personal Mobility Generation} application reaches a comparable level of sophistication by \textit{Iteration 3}.
        \item The \textbf{Mask Adoption Behavior} application exhibits a more gradual and steady evolution, with parameter calibration and model refinement only appearing at \textit{Iterations 4 and 5}.
    \end{itemize}

    \item \textbf{Blank Cells Reflect Dynamic Agent Behavior and Non-Determinism.} The presence of \textbf{blank cells} (i.e., missing functionalities) across different iterations indicates that \ofsocia agentic system does not guarantee deterministic or linear improvement. Instead, agent decisions and feedback-loop adaptations introduce variability into the progression of functionalities, underscoring the stochastic and adaptive nature of \ofsocia code generation process.
\end{enumerate}

It is important to note that by the end of the iterations listed in Table~\ref{tab:simulation_code_iteration}, the simulators generated by \socia for each task had already incorporated the \textbf{majority of their core functionalities}. In practice, additional iterations were conducted beyond those shown, primarily focused on refining and upgrading the simulators based on validation results obtained from the training datasets. These later iterations are not included in Table~\ref{tab:simulation_code_iteration} for brevity. Readers interested in the optimization details of these subsequent iterations are referred to Section~\ref{ssec:detailed_functional_overview_iteration}.

In summary, Table~\ref{tab:simulation_code_iteration} reveals that \socia systematically builds up simulation capabilities through iterative self-evaluation and feedback integration. The staged appearance of functionalities—starting from basic code structure to advanced modeling techniques, demonstrating both the \textbf{robustness} and \textbf{adaptability} of the \socia framework. Moreover, the variation across applications highlights its flexibility in responding to task-specific requirements while following a broadly consistent trajectory of code evolution.

\subsection{Detailed Functional Overview at Each Iteration}
\label{ssec:detailed_functional_overview_iteration}
In this subsection, we present a per-application overview of the functionalities implemented by the automatically generated simulators at each iteration. This qualitative analysis illustrates \ofsocia capability to iteratively evolve code across successive development stages.

In the early stages of code generation, the process tends to be slower due to the frequent occurrence of low-level errors such as syntax issues, empty function bodies, indentation problems, and incorrect file references. To avoid overwhelming the reader with trivial details, we aggregate the initial iterations (e.g., \textbf{iter0–3}) for some of the application. In later stages, where the code becomes more stable and meaningful progress is observed, iterations are presented individually.

\subsubsection{E-Commerce and Retail User Modeling}
\label{sssec:user_modeling_evolve}

Based on a detailed examination of the generated code files, we summarize the implemented functionalities and iterative enhancements at each stage of development.

\begin{itemize}
    \item \texttt{simulation\_code\_iter\_0} - \textbf{Initial Implementation}
    \\ The first version establishes a basic user–product interaction simulation system.
        \begin{itemize}
            \item Core components include:
            \begin{itemize}
                \item A \texttt{User} class representing individuals who can rate and review products.
                \item A \texttt{Product} class that receives reviews and ratings.
                \item A \texttt{Simulation} class that orchestrates the simulation process.
            \end{itemize}  
            \item The rating logic is rudimentary, based on random numbers and simplistic preference models, with no advanced reasoning or personalization.
        \end{itemize}

    \item \texttt{simulation\_code\_iter\_1 - iter\_3} - \textbf{Architecture and Integration}
        \\ Subsequent iterations introduce a modular agent-based architecture:
        \begin{itemize}
            \item \textbf{New components} include:
            \begin{itemize}
                \item \texttt{PlanningAgent}: decomposes high-level tasks into executable steps.
                \item \texttt{MemoryAgent}: stores historical interaction data.
                \item \texttt{ReasoningAgent}: simulates user behavior through rule-based or learned inference.
            \end{itemize}
            \item \textbf{Functional improvements}:
            \begin{itemize}
                \item Enhanced logic for review generation, accounting for user preferences.
                \item Integration with the proprietary LLM API to generate naturalistic review text.
                \item Use of \texttt{try-except} blocks for API error handling and improved data structures (e.g., dictionaries for faster lookups).
                \item Early support for product attribute influence and simple visualization via matplotlib.
                \item Type hinting and code restructuring improve maintainability.
            \end{itemize}
        \end{itemize}

    \item \texttt{simulation\_code\_iter\_4 - iter\_6} - \textbf{Behavior Modeling and Robustness}
        \\ These iterations significantly enhance the simulation’s realism and robustness:
        \begin{itemize}
            \item \textbf{Review generation} is refined with historical context integration, making outputs more coherent and user-specific.
            \item \textbf{Recommendation logic} is improved to better reflect user preferences and product characteristics.
            \item \textbf{Scoring mechanisms} are upgraded to use more realistic distributions (e.g., uniform instead of integer-based random values).
            \item \textbf{Exception handling} is strengthened, including retry mechanisms and more secure API key loading.
            \item \textbf{Platform-level factors} are introduced—e.g., simulations now consider whether reviews occur on Amazon, Goodreads, or Yelp, affecting both content and tone.
        \end{itemize}

    \item \texttt{simulation\_code\_iter\_7 - iter\_9} - \textbf{Evaluation, Personalization, and Finalization}
        \begin{itemize}
            \item \textbf{Evaluation Framework (Iteration 7)}:
            \begin{itemize}
                \item Introduction of a comprehensive evaluation pipeline including ROUGE score computation.
                \item Multiple sampling attempts per review/score generation to improve quality and stability.
                \item Deployment of a dedicated Evaluation Agent.
            \end{itemize}
            \item \textbf{Enhanced Review Semantics (Iteration 8)}:
            \begin{itemize}
                \item Advanced prompt engineering and historical review formatting.
                \item Richer text generation, with sentiment and context-aware scoring.
                \item Preliminary sentiment analysis and data analytics over generated reviews.
            \end{itemize}
            \item \textbf{Final Version (Iteration 9)}:
            \begin{itemize}
                \item Implementation of platform-specific rating guidelines and style references.
                \item Added functionality for analyzing review tone and structure, filtering reviews by category, handling timestamps, and sorting results.
                \item More sophisticated user–product matching logic, incorporating behavioral history and platform norms.
            \end{itemize}
        \end{itemize}
\end{itemize}

Overall Development Trajectory in \textbf{E-Commerce and Retail User Modeling Application}:
\begin{enumerate}
    \item \textbf{Increased Code Complexity}: The codebase evolved from ~167 lines in the initial version to nearly 800 lines in the final version, reflecting significant functional and structural growth.
    \item \textbf{System Intelligence}: The system progressed from using simple random models to leveraging large language models (LLMs) for generating realistic user reviews and scores.
    \item \textbf{Robust Error Handling}: Exception management capabilities were gradually enhanced, improving the system's reliability.
    \item \textbf{Refined User and Product Modeling}: Iterations introduced more nuanced representations of user preferences and product attributes.
    \item \textbf{Evaluation Capability}: A formal evaluation framework was integrated in later stages to assess the quality and coherence of generated outputs.
    \item \textbf{Performance Optimization}: Improvements were made in data handling efficiency and API interaction reliability.
    \item \textbf{Platform-Specific Simulation}: The system incorporated platform-aware behavior, adapting review content and structure to align with conventions observed on Amazon, Goodreads, and Yelp.
\end{enumerate}

This evolving code series exemplifies a progressively refined recommendation system simulation framework. It transitions from a basic random-based model to a sophisticated AI-driven system capable of simulating realistic user behavior and generating high-fidelity interactions within diverse platform contexts.

\subsubsection{Personal Mobility Generation Application}
\label{sssec:llmob_evolve}

Based on a comprehensive analysis of the simulation code across iterations, we summarize the key functionalities and progressive improvements introduced at each stage of development.

\begin{itemize}
    \item \texttt{simulation\_code\_iter\_0 - iter\_3} - \textbf{Foundational Framework and Initial Enhancements}
        \begin{itemize}
            \item The earliest versions (Iterations 0–3) establish the foundational structure of the city-level activity simulation system.
            \item Core components include the implementation of the \texttt{Resident}, \texttt{Location}, and \texttt{SimulationEnvironment} classes.
            \item Basic functionality for simulating individual participation in activities such as shopping, exercising, socializing, working, and resting is introduced.
            \item Initial capabilities also include simple data loading, simulation loop logic, and elementary error handling.
            \item Visualization support is introduced (via matplotlib), alongside the incorporation of a shortest-path computation module (based on Dijkstra’s algorithm).
            \item Additional improvements include enhanced type annotations, the introduction of the \texttt{Organization} class, modeling of transport modes, and visitor attraction mechanisms for locations.
            \item Preliminary evaluation metrics such as step length, step interval, and Jensen-Shannon divergence are implemented, along with basic trajectory tracking and organizational operating logic.
        \end{itemize}

    \item \texttt{simulation\_code\_iter\_4 - iter\_6} - \textbf{Behavioral Refinement and Simulation Expansion}
        \begin{itemize}
            \item These versions focus on enhancing the simulation's realism, modularity, and robustness.
            \item Improvements include:
            \begin{itemize}
                \item Random seed initialization for reproducibility.
                \item Improved file I/O validation and exception handling.
                \item Implementation of real-data and simulated-data extraction functions.
                \item Extension of temporal reasoning for residents and organizations.
                \item Better modeling of motivation and historical behavior patterns.
            \end{itemize}
            \item Simulation fidelity is increased through the addition of resident personas and daily pattern extraction.
            \item A more complex activity participation mechanism is introduced, including explicit start and end times.
            \item New activity types (e.g., dining, studying) and location opening hour checks are incorporated.
            \item The simulation environment’s time management is restructured, and evaluation and visualization modules are significantly enhanced.
        \end{itemize}

    \item \texttt{simulation\_code\_iter\_7 - iter\_9} - \textbf{Intelligent Scheduling and AI Integration}
    \\ These later iterations focus on intelligent behavior generation, AI-assisted personalization, and optimization under spatial constraints:
        \begin{itemize}
            \item Iteration 7 improves commuting logic based on workplace type, infers home and work locations, and introduces POI (point-of-interest) selection functionality.
            \item Iteration 8 integrates large language models (LLMs) via OpenAI API to generate personalized resident profiles and schedules, enhancing realism in individual behavior modeling.
            \item Iteration 9 refines profile generation, activity location extraction, and schedule normalization. Evaluation metric computation and visual analytics are further improved. Also, it introduces location-aware scheduling optimization that considers spatial constraints (e.g., distance between locations), along with final bug fixes and code documentation.
        \end{itemize}
\end{itemize}

Major Directions of Iterative Improvement in \textbf{Personal Mobility Generation Application}:
\begin{enumerate}
    \item \textbf{Functionality Expansion}: The simulation evolved from modeling basic resident activities to supporting a wide range of activity types, organizational behaviors, and spatial attributes.
    \item \textbf{Data Handling Robustness}: Progressive improvements were made in data loading, error handling, and type validation, significantly increasing system reliability.
    \item \textbf{Algorithmic Sophistication}: The simulation progressed from random activity generation to data-driven pattern extraction and eventually LLM-based intelligent inference.
    \item \textbf{Evaluation Framework}: A comprehensive evaluation system was developed, including metrics such as step length, interval, and Jensen-Shannon divergence to assess simulation realism.
    \item \textbf{Visualization Capabilities}: Visualization evolved from basic output plots to complex trajectory diagrams, activity distribution heatmaps, and location network graphs.
    \item \textbf{AI Integration}: In later versions, OpenAI’s LLMs were integrated to generate nuanced resident profiles and personalized schedules, enhancing behavioral diversity and realism.
    \item \textbf{Spatial Constraints}: The final iteration introduced distance-aware optimization of schedules, making the simulation more consistent with real-world urban dynamics.
\end{enumerate}

Through iterative development, the simulation framework advanced from a basic city activity simulator to a sophisticated system integrating AI-driven decision-making, robust evaluation tools, and rich visualization features. Each version introduced targeted improvements, demonstrating a clear trajectory of growth from fundamental components to complex, realistic simulations of urban resident behavior.

\subsubsection{Mask Adoption Behavior Application}
\label{sssec:mask_evolve}

We analyze the functionality and iterative optimization of each simulation script in this simulation application.

\begin{itemize}
    \item \texttt{simulation\_code\_iter\_0} - \textbf{Baseline Model}
        \begin{itemize}
            \item \textbf{Core Functionality}: Implements a basic mask-wearing behavior diffusion model.
            \item \textbf{Key Components}:
            \begin{itemize}
                \item \texttt{Person} class: Represents individuals with attributes such as mask-wearing status, risk perception, and social network connections.
                \item \texttt{SocialNetwork} class: Defines the structure of the social network.
                \item \texttt{Simulation} class: Manages simulation setup, execution, and evaluation.
            \end{itemize}
            \item \textbf{Basic Features}:
            \begin{itemize}
                \item Simple decision-making model based on social influence and risk perception.
                \item A single type of social connection.
                \item Basic visualization capabilities.
            \end{itemize}
        \end{itemize}

    \item \texttt{simulation\_code\_iter\_1} - \textbf{Error Handling and Parameter Improvements}
        \\ Main Enhancements:
        \begin{itemize}
            \item Improved error handling to account for more exceptional cases.
            \item Migration of key parameters (e.g., influence probability, risk perception effect) into the Person class.
            \item Refined computation of social influence by incorporating behavioral differences.
            \item Strengthened data validation, including file format and data type checks.
        \end{itemize}

    \item \texttt{simulation\_code\_iter\_2} - \textbf{Visual Analytics and Detailed Reporting}
        \\ Key Enhancements:
        \begin{itemize}
            \item Added a mechanism for dynamic decay of social influence over time.
            \item Introduced a \texttt{calibrate\_parameters} method for model parameter tuning.
            \item Significant upgrades to visualization: Multiple chart types (e.g., histograms, scatter plots); Analysis of mask-wearing rates grouped by risk perception.
            \item More comprehensive output reporting and terminal summaries.
            \item Initial implementation of simulated government interventions.
        \end{itemize}

    \item \texttt{simulation\_code\_iter\_3} - \textbf{Complex Behavioral Modeling}
        \\ Model Refinement:
        \begin{itemize}
            \item Introduced a habit formation mechanism to capture behavioral consistency.
            \item Added dynamic decision thresholds at the individual level.
            \item Improved the social influence model by including: Reinforcement of similar behaviors (echo chamber effect); Environmental risk factors; Special handling for high-risk individuals.
            \item Implemented a two-phase behavior propagation process: first calculate all influence updates, then apply them collectively.
        \end{itemize}

    \item \texttt{simulation\_code\_iter\_4} - \textbf{Code Refactoring and Parameter Calibration}
        \\ Functional Optimizations:
        \begin{itemize}
            \item Introduced a sigmoid function for smoother decision modeling.
            \item Refactored the codebase to improve naming conventions and structure.
            \item Developed detailed parameter calibration logic: Estimated risk perception effects using training data; Computed information diffusion rate from daily behavioral change; Derived social network influence weights from state transitions.
            \item Improved code readability through enhanced comments and documentation.
        \end{itemize}

    \item \texttt{simulation\_code\_iter\_5} - \textbf{Advanced Social Network and Personalization}
        \\ Major Upgrades:
        \begin{itemize}
            \item Differentiated types of social ties (e.g., family, workplace/school, community) with assigned weights.
            \item Implemented clustering mechanisms to segment the population based on key features.
            \item Enabled cluster-specific parameters for more distinct behavior patterns across groups.
            \item Incorporated memory effects, allowing past decisions to influence current behavior.
            \item Added an intervention fatigue mechanism to simulate declining effectiveness of long-term policies.
            \item Integrated a more complex decision-making model combining multiple factors with probabilistic decisions.
            \item Introduced advanced visualization features, including cluster-based analysis and dynamic environmental risk overlays.
        \end{itemize}
\end{itemize}

Summary of Iterative Optimization in \textbf{Mask Adoption Behavior Application}:
\begin{enumerate}
    \item Began with a simple social network and decision-making framework.
    \item Gradually introduced complexity through error handling, parameter tuning, and visual analysis.
    \item Incorporated realistic behavioral mechanisms such as habit formation, echo chamber effects, and environmental influences.
    \item Applied mathematical modeling enhancements, including sigmoid functions and probabilistic reasoning.
    \item Ultimately arrived at a highly personalized simulation model with diverse connection types, population clustering, memory effects, and adaptive behaviors.
\end{enumerate}
Each version addressed the limitations of its predecessor and added new capabilities, progressively constructing a more realistic and sophisticated simulation system for modeling mask-wearing behavior diffusion.
