# Supplementary material for: SOCIA-$\nabla$: Textual Gradient Meets Multi-Agent Orchestration for Automated Simulator Generation
Source: arXiv:2505.12006 source file (2026-11-04)
Supplement: Supplementary file 6 [file 6_task_brief.tex]

In this section, we provide an illustrative example of a complete task brief generated by the \textbf{Data Analysis Agent} for the \textbf{Mask Adoption Behavior} scenario. This structured JSON object contains all the necessary information, from data analysis summaries to simulation design parameters, required by downstream agents to construct and execute the simulator.

\begin{AIBoxBreak}{Generated Task Brief: Mask Adoption Behavior}
\begin{lstlisting}[breaklines=true]
{
  "title": "Simulation Task",
  "description": "Develop a multi-agent simulation system that models the spread of mask-wearing behavior through social networks.",
  "simulation_focus": [
    "Predict agents' mask-wearing behavior over day 30 - day 39 (last ten days) based on their attributes, social connections, and past behavior",
    "Model information propagation and behavioral changes triggered by social influence and government intervention starting on Day 10"
  ],
  "data_folder": "data_fitting/mask_adoption_data/",
  "data_files": {
    "agent_attributes.csv": "Contains demographic and behavioral attributes of each agent, including age, occupation, risk perception, and social connection counts",
    "social_network.json": "Contains structured data representing a social network. Each entry corresponds to a user (identified by a unique integer ID), and the values describe the different types of relationships that user has with others. Data Structure: The top-level structure is a dictionary ({} in JSON). Keys: Each key is a unique user ID (as an integer, e.g., 0, 1, 2, etc.). Values: Each value is another dictionary with the following fields: \"family\": a list of user IDs representing family connections. \"work_school\": a list of user IDs representing colleagues or schoolmates. \"community\": a list of user IDs representing community-level acquaintances. \"all\": a merged list of all user IDs connected to the user across the three categories above.",
    "train_data.csv": "Time series data for the first 30 days, used for training the model"
  },
  "evaluation_metrics": {
    "RMSE": {
      "description": "Root Mean Square Error measuring overall predictive accuracy of mask adoption rates",
      "interpretation": "Directly interpretable as percentage deviations due to the 0-1 range",
      "formula": "RMSE = sqrt(sum((predicted_rate - actual_rate)^2) / n)"
    }
  },
  "data_analysis_result": {
    "overall_simulation_design": {
      "objective": "Model and forecast the spread and persistence of mask-wearing behavior across a multilayer social network via social influence, individual risk perception, and exogenous information signals; automatically calibrate behavioral parameters to longitudinal observations.",
      "initialization": "1) Load agents from agent_attributes.csv (IDs, demographics, risk_perception, initial_mask_wearing). 2) Load network from social_network.json; build multiplex layers (family, work_school, community), symmetrize and deduplicate edges. 3) Align populations across files; use intersection of IDs. 4) Set day 0 mask state per agent from train_data.csv when available; otherwise fallback to initial_mask_wearing. 5) Derive initial received_info from train_data day 0 if provided; else initialize false. 6) Precompute per-agent layer degrees and normalization constants. 7) Initialize parameter vector (layer weights, inertia, risk sensitivity, info diffusion, exogenous broadcast rate, decay) with priors or heuristic defaults.",
      "execution": "Daily synchronous updates. At each time step, compute per-agent neighbor mask share per layer; generate received_info via peer and exogenous channels; compute mask adoption probability using a calibrated logistic decision rule with inertia and demographics. Calibrate parameters by maximizing the likelihood of observed wearing_mask transitions on the training time window (penalized logistic regression over panel data) while matching observed received_info rates; use gradient-based optimization or Bayesian optimization with cross-validated early stopping. After calibration, run forward simulations on the validation window from the last observed state, then evaluate.",
      "outputs": [
        "Calibrated parameter set (point estimates and, if enabled, posterior samples/uncertainty)",
        "Validation forecasts of per-agent and aggregate mask-wearing trajectories",
        "Evaluation metrics on validation set (RMSE, MAE, Brier, TransitionFit)",
        "Calibration diagnostics (convergence stats, parameter sensitivities, regularization paths)",
        "Reproducible seeds and configuration used for this run"
      ]
    },
    "scale_granularity": {
      "time_step": "days",
      "spatial_resolution": "non-spatial",
      "population_size": "Number of unique agent_id present in both agent_attributes.csv and social_network.json (expected ~1000 based on samples)",
      "rationale": "train_data.csv is daily; network interactions are not spatially explicit; population equals provided social graph."
    },
    "agent_archetypes": {
      "unit": "resident",
      "roles": [
        "resident",
        "campaign_broadcaster"
      ],
      "static_attributes": [
        "agent_id",
        "age",
        "age_group",
        "occupation",
        "risk_perception",
        "layer_degrees: family_connections, work_school_connections, community_connections",
        "demographic multipliers (derived, not raw fields)"
      ],
      "dynamic_states": [
        "wearing_mask_t (bool)",
        "received_info_t (bool)",
        "memory_of_info_t (continuous 0-1, optional for decay)",
        "propensity_score_t (latent probability from decision rule)"
      ],
      "construction_from_data": "Map each CSV row in agent_attributes.csv to an agent. Set initial wearing_mask_t from train_data day 0 if available, else from initial_mask_wearing. Risk perception is the provided [0,1] value. Age group and occupation are categorical features used as fixed effects or multipliers. Degrees per layer come from agent_attributes.csv for validation; actual edges come from social_network.json.",
      "update_from_data": "During calibration, use train_data.csv to compute observed transitions (wear_t-1 -> wear_t) and received_info_t targets per day-agent. These observations fit the logistic decision model to estimate parameters. During simulation, dynamic states update from the model using simulated signals (neighbor influence and exogenous info) and the last state."
    },
    "interaction_topology": {
      "topology": "graph",
      "layers": [
        "family",
        "work_school",
        "community",
        "all (union, optional projection)"
      ],
      "protocol": "peer-to-peer interactions on each layer with layer-specific weights; synchronous daily update of states",
      "construction_from_data": "Use social_network.json adjacency lists per agent per layer. Symmetrize edges (if i lists j, ensure j lists i) and remove duplicates. Validate node IDs against agent_attributes.csv. If social_network.json is unavailable for some IDs, optionally synthesize edges using the degree targets in agent_attributes.csv via a configuration-model per layer respecting plausible homophily (e.g., students in work/school)."
    },
    "information_propagation": {
      "exists": true,
      "topology": "Multiplex diffusion across family, work_school, community; plus global broadcast channel",
      "mechanism": "Each day, an agent receives information with probability: 1 - exp(-(phi_family * share_family - weighted by mask-wearing neighbors - + phi_work * share_work + phi_community * share_community + lambda_broadcast)), capped at [0,1]. Optionally maintain a decaying memory_of_info with rate rho_info_decay that sustains influence for several days.",
      "construction_from_data": "If train_data.csv includes received_info, match the empirical daily and agent-level prevalence to calibrate lambda_broadcast and phi_* via likelihood or moment matching. If received_info is missing or sparse, infer via the peer mechanism only and calibrate to reproduce mask adoption dynamics.",
      "parameters": {
        "names": [
          "phi_family",
          "phi_work",
          "phi_community",
          "lambda_broadcast",
          "rho_info_decay"
        ],
        "notes": "phi_* scale peer info exposure per layer; lambda_broadcast is a daily rate for exogenous campaigns; rho_info_decay controls persistence of received_info. Estimate from observed received_info (if present) and mask transitions via joint likelihood."
      }
    },
    "exogenous_signals": [
      {
        "name": "received_info_broadcast",
        "construction_from_data": "train_data.csv received_info field and its daily prevalence; if absent, treat as latent and calibrate lambda_broadcast to fit adoption curves.",
        "observability": "Residents can observe their own exposure; no delay assumed; can include binomial noise.",
        "effect_on_agents": "Adds an exogenous term to adoption probability and reduces abandonment probability (enters decision rule as a positive coefficient).",
        "bounds": "[0,1] daily probability"
      }
    ],
    "action_decision_policy": {
      "by_role": {
        "resident": {
          "inputs": [
            "previous wearing_mask state",
            "neighbor mask share per layer (family, work_school, community)",
            "risk_perception",
            "received_info (current or decayed memory)",
            "demographic indicators: age_group, occupation",
            "degree-normalized influence (optional)"
          ],
          "policy_form": "Logistic adoption-retention model. Let x_t be a feature vector including: intercept; inertia I(wear_t-1); neighbor shares per layer weighted by w_family, w_work, w_community; risk_perception; received_info (or memory); demographic fixed effects; interaction terms (e.g., risk_perception * received_info). Adoption probability P(wear_t=1 | x_t) = sigmoid(alpha + gamma*I(wear_t-1) + beta_f*w_family*share_family + beta_w*w_work*share_work + beta_c*w_community*share_community + beta_r*risk + beta_i*received_info + demographic terms). State is sampled Bernoulli from this probability (or use deterministic threshold for expectation runs).",
          "parameters": [
            "alpha (intercept)",
            "gamma (inertia/persistence)",
            "w_family, w_work, w_community (layer weights, sum-to-one constraint applied during calibration)",
            "beta_f, beta_w, beta_c (peer influence slopes per layer)",
            "beta_r (risk perception coefficient)",
            "beta_i (info exposure coefficient)",
            "age_group effects: beta_age_youth, beta_age_young_adult, beta_age_middle_age, beta_age_senior (one is baseline)",
            "occupation effects: beta_occ_student, beta_occ_blue_collar, beta_occ_white_collar (one baseline)",
            "tau (temperature/noise scaling, optional)"
          ]
        },
        "campaign_broadcaster": {
          "inputs": [
            "target coverage or budget (optional)",
            "current adoption rate (optional for feedback control)"
          ],
          "policy_form": "Stateless stochastic broadcast: each agent independently receives info with probability lambda_broadcast per day; optionally modulate lambda_broadcast by time or adoption level.",
          "parameters": [
            "lambda_broadcast"
          ]
        }
      }
    },
    "holdout_plan": {
      "method": "temporal_holdout",
      "train_range": "First 80% of days per agent in train_data.csv (e.g., if days 0-99, train on 0-79).",
      "validation_range": "Last 20% of days per agent (e.g., days 80-99).",
      "notes": "Initialize validation simulation from the last observed train-day state per agent. Ensure no leakage of validation labels into calibration of parameters."
    },
    "simulation_evaluation": {
      "metrics": [
        {
          "name": "RMSE_aggregate",
          "definition": "Root Mean Squared Error between simulated and observed daily population-level mask-wearing rates on validation days."
        },
        {
          "name": "MAE_aggregate",
          "definition": "Mean Absolute Error between simulated and observed daily adoption rates on validation."
        },
        {
          "name": "Brier",
          "definition": "Mean squared error between predicted per-agent probabilities and observed wearing_mask outcomes on validation."
        },
        {
          "name": "TransitionFit",
          "definition": "Absolute or squared error between simulated and observed transition probabilities P01, P11, P10, P00 on validation."
        }
      ],
      "comparison_method": "Run K stochastic simulations on the validation window (e.g., K=50) and average metrics; report mean+/-CI. Also report calibration plots: simulated vs observed aggregate curve, and confusion/transition matrices. Select best run by mean Brier or a weighted composite of metrics."
    },
    "calibratable_parameters": [
      {
        "name": "w_family, w_work, w_community",
        "range_bounds": "[0, 2] each; normalized to sum to 1 at runtime",
        "source": "Layer salience; constrained by network layers and observed dynamics",
        "notes": "Higher family weight typically increases clustering-driven adoption."
      },
      {
        "name": "beta_f, beta_w, beta_c",
        "range_bounds": "[0, 5]",
        "source": "Peer influence slopes per layer from train_data transitions",
        "notes": "Control sensitivity to neighbor mask share."
      },
      {
        "name": "gamma (inertia)",
        "range_bounds": "[0, 6]",
        "source": "Persistence of behavior",
        "notes": "Higher gamma reduces switching; calibrated from P11 and P00."
      },
      {
        "name": "beta_r (risk perception coefficient)",
        "range_bounds": "[0, 5]",
        "source": "agent_attributes.risk_perception",
        "notes": "Scales individual propensity to wear independent of peers."
      },
      {
        "name": "beta_i (info exposure effect)",
        "range_bounds": "[0, 5]",
        "source": "train_data.received_info",
        "notes": "Amplifies adoption when exposed to information."
      },
      {
        "name": "lambda_broadcast",
        "range_bounds": "[0, 0.5] daily",
        "source": "Exogenous info prevalence in train_data",
        "notes": "Baseline probability of receiving info independent of peers."
      },
      {
        "name": "phi_family, phi_work, phi_community",
        "range_bounds": "[0, 2]",
        "source": "Information propagation via peers",
        "notes": "Map neighbor mask share to info receipt probability."
      },
      {
        "name": "rho_info_decay",
        "range_bounds": "[0, 1]",
        "source": "Duration of info effect",
        "notes": "Per-day retention of received_info memory."
      },
      {
        "name": "alpha (intercept)",
        "range_bounds": "[-5, 5]",
        "source": "Baseline adoption propensity",
        "notes": "Centers probabilities absent other signals."
      },
      {
        "name": "age_group effects (beta_age_*)",
        "range_bounds": "[-3, 3]",
        "source": "agent_attributes.age_group",
        "notes": "Additive fixed effects; one category is baseline at 0."
      },
      {
        "name": "occupation effects (beta_occ_*)",
        "range_bounds": "[-3, 3]",
        "source": "agent_attributes.occupation",
        "notes": "Additive fixed effects; one category baseline."
      },
      {
        "name": "tau (temperature/noise)",
        "range_bounds": "[0.5, 5]",
        "source": "Controls stochasticity in decision sampling",
        "notes": "Lower tau yields more deterministic behavior."
      },
      {
        "name": "regularization (L2)",
        "range_bounds": "[0, 10]",
        "source": "Calibration stabilization",
        "notes": "Prevents overfitting; tuned by inner CV on train window."
      }
    ]
  }
}
\end{lstlisting}
\end{AIBoxBreak}
